# Supplementary material for: Hopf categories and the categorification of the Heisenberg algebra via graphical calculus
Source: arXiv:1612.06911 source file (2016-12-20)
Supplement: Supplementary file 1 [file appendix.tex]

\appendix
\section{Commutative cubes}
\label{app:commcube}
In this section we explain what we mean by the term "commutative cube" in a bicategory. The general statement is as follows: for an $n$-dimensional cube given an ordering of the coordinates there is a concise way to orient the 2-morphisms, thus getting a diagram of 2-morphisms for any cube. We will say that the cube is commutative if this diagram is. The ordering used in this article is described below. A good general reference for this topic is \cite{graycoherence}. 

\subsection{2-cubes}

Consider a square, where we have ordered the coordinates as $x<y$. Then we orient the 2-morphism by the lexicographical order, i.e. $xy\rightarrow yx$.

\begin{align*}
\stik{1}{
{} \ar{r}{x} \ar{d}{y} \& {}\\
{} \& {}
}
&
{}
&
\stik{1}{
{} \ar{r}{x} \ar{d}[left]{y}\& {} \ar{d}{y}\ar[Rightarrow,shorten <=1em,shorten >=1em]{dl}[above,sloped]{}\\
{} \ar{r}[below]{x}\& {}
}
\end{align*}

\subsection{3-cubes}
Order the three coordinates in the cube as $x<y<z$. The edges of the cube are all oriented positively in one of these directions, i.e. as in the diagram:
\[\stik{1}{
{} \& {} \ar{rr} \ar{dd} \& {} \& {} \ar{dd}\\
{} \ar[crossing over]{rr}[xshift=1pc]{x} \ar{dd}{y} \ar{ur}{z} \& {} \& {} \ar{dd}{} \ar{ur} \& {}\\
{} \& {} \ar{rr} \& {} \& {}\\
{} \ar{rr} \ar{ur} \& {} \& {} \ar{ur}
\latearrow{commutative diagrams/crossing over}{2-3}{4-3}{}
}
\]
The 2-morphisms are oriented as in the previous section. E.g. we have a morphism $xy\rightarrow yx$, and via whiskering we get a morphism $xyz\rightarrow  yxz$.

In this way we get a diagram of all 2-morphisms between full paths on the cube, which is a hexagon
\begin{equation}
\label{app:2morphoncube}
\stik{1}{
\& yxz \ar{r} \& yzx \ar{dr}\\
xyz \ar{ur} \ar{dr} \& \& \& zyx\\
\& xzy \ar{r}\& zxy \ar{ur}
}
\end{equation}

We say that the cube is commutative if this diagram commutes.

We can draw this diagram in the cube in the following way:
\begin{align*}
\stik{0.7}{
{} \& {} \& {}\\
{} \ar{ur}{\scalebox{2}{$z$}} \ar{rr}{\scalebox{2}{$x$}} \ar{dd}{\scalebox{2}{$y$}} \& {} \& {}\\
{} \& {} \& {} \\
{} \& {} \& {}
}
&
{}
&
\stik{0.7}{
{} \& {} \ar{rr}[name=topback,below]{} \ar{dd}[name=backleft,sloped,xshift=-1.5pc]{} \& {} \& {} \ar{dd}\\
{} \ar[crossing over]{rr}[name=topfront,above]{}\ar{dd}[name=frontleft]{} \ar{ur}[name=topleft,below]{} \& {} \& {} \ar{dd}[name=frontright,sloped,xshift=1pc]{} \ar{ur}[name=topright,below]{} \& {}\\
{} \& {} \ar{rr} \& {} \& {}\\
{} \ar{rr}[name=bottomfront,below]{} \ar{ur}[name=bottomleft,sloped,yshift=-0.2pc]{} \& {} \& {} \ar{ur}
\arrow[Rightarrow,to path={(topright) to[bend left] (topback)}]{}{}
\arrow[Rightarrow,to path={(frontright) to[bend right] (bottomfront)}]{}{}
\arrow[Rightarrow,crossing over,to path={(frontright) to[bend right] (topright)}]{}{}
\arrow[Rightarrow,to path={(bottomfront) to[bend right] (bottomleft)}]{}{}
\arrow[Rightarrow,to path={(bottomleft) to[bend left] (backleft)}]{}{}
\arrow[Rightarrow,to path={(topback) to[bend left] (backleft)}]{}{}
\latearrow{/tikz/commutative diagrams/crossing over}{2-3}{4-3}{}
\latearrow{/tikz/commutative diagrams/crossing over}{2-1}{2-3}{}
\latearrow{/tikz/commutative diagrams/crossing over}{2-3}{1-4}{}
}
\end{align*}

\begin{Lemma}
\label{lem:cubefront}
\label{app:cubecommutes}
Consider a cube in a bicategory:
\[\stik{1}{
{} \& {} \ar{rr}{x} \ar{dd}[left,yshift=-1pc]{y} \& {} \& {} \ar{dd}{y}\\
{} \ar[crossing over]{rr}[xshift=1pc]{x} \ar{dd}[left]{y} \ar{ur}{z} \& {} \& {} \ar{dd}[yshift=-1pc,left,xshift=-0.5pc]{y} \ar{ur}{z} \& {}\\
{} \& {} \ar{rr}[xshift=-1pc]{x} \& {} \& {}\\
{} \ar{rr}{x} \ar{ur}{z} \& {} \& {} \ar[equal]{ur}
\latearrow{commutative diagrams/crossing over}{2-3}{4-3}{}
}
\]
with all faces given except the front, and such that the left and bottom faces are invertible, then there is a unique 2-morphism that fits in the front face and makes the cube commute.
\end{Lemma}
\begin{proof}
The graph of 2-morphisms is
\[
\stik{1}{
\& yx \ar{r}[sloped]{\sim} \& yzx \ar{dr}[sloped]{\sim}\\
xy \ar{ur}[sloped]{\alpha} \ar{dr} \& \& \& zyx\\
\& xzy \ar{r}\& zxy \ar{ur}
}
\]
so the morphism $\alpha:xy\rightarrow yx$ that makes this diagram commute exists and is unique.
\end{proof}

\subsection{Higher dimensional cubes}
In the same way we can orient the 2-morphisms on any $k$-cube by ordering the coordinates as $x_1,\ldots,x_k$.

For instance for a 4-cube the resulting diagram is a 3-dimensional shape with 8 faces which are hexagons and 6 faces which are squares (a \emph{truncated octahedron}). The entire diagram commutes iff each face commutes. The hexagons correspond to the sub 3-cubes, and the squares are related to the four-interchange law in a bicategory. So we see that a 4-cube in a bicategory commutes iff every sub 3-cube in it commutes.

More generally we have
\begin{Theorem}[Gray, \cite{graycoherence}]
A $k$-cube in a bicategory commutes iff every sub 3-cube in it commutes.
\end{Theorem}
%%%%%%%%%%%%%%%%%%%%%%%%%%%%%%%%%%%%%%%%%%%%%%%%%%%%%
%%%%%%%%%%%%%%%%%%%%%%%%%%%%%%%%%%%%%%%%%%%%%%%%%%%%%
\subsection{Computation for \autoref{proof:cartesianBC}}
\label{app:4cubecomputation}
We need to show that the front cube commutes.

The front cube is 
\[
\stik{1}{
{} \& M \ar{rr}[name=topback,below]{}[above]{} \ar{dd}[name=backleft,sloped,xshift=-1.5pc]{}[right,yshift=-1.5pc]{C_R} \& {} \& B \ar[equal]{dd}\\
M \ar[crossing over]{rr}[name=topfront,above]{}[below, xshift=1pc]{} \ar{dd}[name=frontleft]{}[left]{Y} \ar[equal]{ur}[name=topleft,below]{} \& {} \& B \ar[equal]{dd}[name=frontright,sloped,xshift=1pc]{} \ar[equal]{ur}[name=topright,below]{} \& {}\\
{} \& A \ar{rr} \& {} \&B\\
A \ar{rr}[name=bottomfront,below]{} \ar[equal]{ur}[name=bottomleft,sloped,yshift=-0.2pc]{} \& {} \& B \ar[equal]{ur}
\arrow[equal,to path={(topright) to[bend left] (topback)}]{}{}
\arrow[Rightarrow,to path={(frontright) to[bend right] (bottomfront)},"g_Y"]{}{}
\arrow[equal,crossing over,to path={(frontright) to[bend right] (topright)}]{}{}
\arrow[equal,to path={(bottomfront) to[bend right] (bottomleft)}]{}{}
\arrow[Rightarrow,to path={(bottomleft) to[bend left] (backleft)},"\psi"]{}{}
\arrow[Rightarrow,to path={(topback) to[bend left] (backleft)},"g_R"']{}{}
\latearrow{commutative diagrams/crossing over,commutative diagrams/equal}{2-3}{4-3}{}
\latearrow{commutative diagrams/crossing over}{2-1}{2-3}{}
\latearrow{commutative diagrams/crossing over,commutative diagrams/equal}{2-3}{1-4}{}
}
\]
So we need to show that $\psi\circ g_Y=g_R$.

Recall that
\[
g_R=\nstik{1}{
{} \ar{d}{b} \& \ar{d}{b} \ar[yshift=-1em,shorten <=1em,shorten >=0.2em]{dr}[xshift=0em]{\beta} \& \ar{d}{a} \& \ar{d}{a}\\
{} \ar[equal]{d} \ar[yshift=-1em,shorten <=1em,shorten >=0.2em]{dr}[xshift=-0.5em]{\eta} \& \ar{d}{g} \ar[yshift=-1.5em,shorten <=1.2em]{ur} \& \ar{d}{f} \ar[yshift=-1em,shorten <=1em,shorten >=0.2em]{dr}[xshift=0em]{\alpha_R^{-1}} \& \ar{d}{i_R}\\
{} \ar[equal]{d} \ar[yshift=-1.5em,shorten <=1.2em]{ur} \& \ar{d}{g_R} \& \ar{d}{g_R} \ar[yshift=-1.5em,shorten <=1.2em]{ur} \& \ar{d}{h}\\
{} \& {} \& {} \& {}
}
\]
Denoting the front face of the outer cube (the "$Y$"-cube ) by $g_Y$, we have $\beta=f_Y\circ\alpha\circ g_Y$.

Substituting we get
\[g_R=
\nstik{1}{
{} \ar{dd}{b} \& \ar{dd}{b} \ar[yshift=-1em,shorten <=1em,shorten >=0.2em]{dr}[xshift=0em]{g_Y}\& \ar{d}{Y} \& \ar{d}{Y} \ar[yshift=-1em,shorten <=1em,shorten >=0.2em]{dr}[xshift=0em]{f_Y}\& \ar{dd}{a} \& \ar{dd}{a}\\
{} \& {} \ar[yshift=-1.5em,shorten <=1.2em]{ur} \& \ar{d}{h} \ar[yshift=-1em,shorten <=1em,shorten >=0.2em]{dr}[xshift=-0.5em]{\alpha}\& \ar{d}{i} \ar[yshift=-1.5em,shorten <=1.2em]{ur}\& {}\& {}\\
{} \ar[equal]{d} \ar[yshift=-1em,shorten <=1em,shorten >=0.2em]{dr}[xshift=-0.5em]{\eta} \& \ar{d}{g}  \& \ar{d}{g} \ar[yshift=-1.5em,shorten <=1.2em]{ur}  \& \ar{d}{f} \& {} \ar{d}{f} \ar[yshift=-1em,shorten <=1em,shorten >=0.2em]{dr}[xshift=0em]{\alpha_R^{-1}} \& {} \ar{d}{i_R}\\
{} \ar[equal]{d} \ar[yshift=-1.5em,shorten <=1.2em]{ur} \& \ar{d}{g_R} \& \ar{d}{g_R}  \& {} \ar{d}{g_r} \& {} \ar{d}{g_R} \ar[yshift=-1.5em,shorten <=1.2em]{ur} \& {} \ar{d}{h}\\
{} \& {} \& {} \& {} \& {} \& {}
}
\]

Now we plug in the identity of $i$ in the fourth column as a composition of unit/counit maps, and interchange $g_Y$ and $\eta$:
\[g_R=
\nstik{0.95}{
{} \& {} \& {} \& {}\ar{d}{Y} \& {} \ar{d}{Y} \& {} \ar{d}{Y} \ar[yshift=-1em,shorten <=1em,shorten >=0.2em]{dr}[xshift=0em]{f_Y}\& {}\ar{dd}{a} \& {}\ar{dd}{a}\\
{} \& {} \& {} \& {}\ar[yshift=-1em,shorten <=1em,shorten >=0.2em]{dr}[xshift=0em]{\eta'}\ar[equal]{dd} \& {} \ar{d}{i} \& {} \ar{d}{i} \ar[yshift=-1.5em,shorten <=1.2em]{ur} \& {} \& {}\\
{} \ar{dd}{b} \ar[yshift=-1em,shorten <=1em,shorten >=0.2em]{dr}[xshift=0em]{g_Y} \& \ar{d}{Y} \& \ar{d}{Y} \& {} \ar[yshift=-1.5em,shorten <=1.2em]{ur} \& {} \ar{d}{i_R} \ar[yshift=-1em,shorten <=1em,shorten >=0.2em]{dr}[xshift=0em]{\epsilon'}\& {} \ar[equal]{dd} \& {}  \ar[equal]{dd} \& \ar[equal]{dd}\\
{} \ar[yshift=-1.5em,shorten <=1.2em]{ur} \& {}\ar{d}{h} \& {}\ar{d}{h} \ar[yshift=-1em,shorten <=1em,shorten >=0.2em]{dr}[xshift=-0.5em]{\alpha}\& {}\ar{d}{i} \& {} \ar{d}{i} \ar[yshift=-1.5em,shorten <=1.2em]{ur} \& {}\& {}\& {}\\
{} \ar[equal]{dd}  \& {} \ar[equal]{dd} \ar[yshift=-1em,shorten <=1em,shorten >=0.2em]{dr}[xshift=-0.5em]{\eta} \& \ar{d}{g} \ar[yshift=-1.5em,shorten <=1.2em]{ur}  \& \ar{d}{f} \& {} \ar{d}{f}  \& {} \ar{d}{f} \& {}\ar{d}{f}  \ar[yshift=-1em,shorten <=1em,shorten >=0.2em]{dr}[xshift=0em]{\alpha_R^{-1}}\& {}\ar{d}{i_R} \\
{}  \& \ar[yshift=-1.5em,shorten <=1.2em]{ur} \& \ar{d}{g_R}  \& {} \ar{d}{g_r} \& {} \ar{d}{g_R}  \& {} \ar{d}{g_R}\& {}\ar{d}{g_R} \ar[yshift=-1.5em,shorten <=1.2em]{ur}\& {} \ar{d}{h}\\
{} \& {} \& {} \& {} \& {} \& {}\& {} \& {}
}
\]

using some interchanging we get to
\[g_R=
\nstik{0.95}{
{} \& {}\ar{d}{Y} \& {}\ar{d}{Y} \& {}\ar{d}{Y} \& {} \ar{d}{Y} \& {} \ar{d}{Y} \& {}\ar{d}{Y} \ar[yshift=-1em,shorten <=1em,shorten >=0.2em]{dr}[xshift=0em]{f_Y} \& {}\ar{dd}{a}\\
{} \& {}\ar[equal]{dd} \ar[yshift=-1em,shorten <=1em,shorten >=0.2em]{dr}[xshift=0em]{\eta'} \& {} \ar{d}{i} \& {} \ar{d}{i} \& {} \ar{d}{i} \& {} \ar{d}{i}  \& {}\ar{d}{i}\ar[yshift=-1.5em,shorten <=1.2em]{ur} \& {}\\
{} \ar{dd}{b} \ar[yshift=-1em,shorten <=0em,shorten >=0.2em]{dr}[xshift=0em]{g_Y} \& {} \ar[yshift=-1.5em,shorten <=1.2em]{ur} \& {} \ar{d}{i_R} \& {}  \ar{d}{i_R} \& {} \ar{d}{i_R} \ar[yshift=-1em,shorten <=1em,shorten >=0.2em]{dr}[xshift=0em]{\epsilon'}\& {} \ar[equal]{dd} \& {}  \ar[equal]{dd} \& \ar[equal]{dd}\\
{} \ar[yshift=-1.5em,shorten <=1.2em]{uuur} \& {}\ar{d}{h} \& {}\ar{d}{h} \& {} \ar[yshift=-1em,shorten <=1em,shorten >=0.2em]{dr}[xshift=-0.5em]{\alpha} \ar{d}{h} \& {} \ar{d}{i} \ar[yshift=-1.5em,shorten <=1.2em]{ur} \& {}\& {}\& {}\\
{} \ar[equal]{dd}  \& {} \ar[equal]{dd}  \& {} \ar[equal]{dd} \ar[yshift=-1em,shorten <=1em,shorten >=0.2em]{dr}[xshift=-0.5em]{\eta}   \& \ar{d}{g} \ar[yshift=-1.5em,shorten <=1.2em]{ur} \& {} \ar{d}{f}  \& {} \ar{d}{f}\ar[yshift=-1em,shorten <=1em,shorten >=0.2em]{dr}[xshift=0em]{\alpha_R^{-1}} \& {}\ar{d}{i_R}  \& {}\ar{d}{i_R} \\
{}   \& {} \& {} \ar[yshift=-1.5em,shorten <=1.2em]{ur} \& {} \ar{d}{g_R} \& {} \ar{d}{g_R}  \& {} \ar{d}{g_R} \ar[yshift=-1.5em,shorten <=1.2em]{ur} \& {}\ar{d}{h} \& {} \ar{d}{h}\\
{} \& {} \& {} \& {} \& {} \& {}\& {} \& {}
}
\]

Finally, we can cancel the middle part, which is just $\alpha_R^{-1}\circ\alpha_R$ and get \[
g_R=f_Y\circ \eta'\circ g_Y=\psi\circ g_Y
\]
as required.
%%%%%%%%%%%%%%%%%%%%%%%%%%%%%%%%%%%%%%%%%%%%%%%%%%%%%
%%%%%%%%%%%%%%%%%%%%%%%%%%%%%%%%%%%%%%%%%%%%%%%%%%%%%
\section{The Beck-Chevalley condition for squares and cubes}
\label{sec:BC}
\label{app:BeckChevalley}
Let $\CCC$ be a bicategory, and consider a square (sometimes called a \emph{quintet})
\begin{equation}
\label{bcsquarebefore}
\tik
A\arrow[]{d}{f} \arrow[]{r}{g}& B \arrow[]{d}{h} \arrow[shorten >=0.4cm,shorten <=0.4cm,Rightarrow]{dl}[above,sloped]{\alpha} \\ 
C \arrow[]{r}{i} & D
\tak
\end{equation}
i.e. a 2-morphism $\alpha:h\circ g\rightarrow i\circ f$ (which is not necessarily an isomorphism).

Suppose that the verticals $h,f$ both have right adjoints $h_R,f_R$, with given unit-counit pairs, then we can form the square (called the \emph{right mate} of the above square)
\[
\tik
A \arrow[]{r}{g}\arrow[blue,shorten >=0.4cm,shorten <=0.4cm,Rightarrow]{dr}[above,sloped]{\alpha_R}& B   \\ 
C \arrow[dashed,blue,thick]{u}{f_R} \arrow[]{r}{i} & D \arrow[dashed,blue,thick]{u}[right]{h_R}
\tak
\]
where $\alpha_R$ is the composition
\[
g\circ f_R\rightarrow h_R\circ h \circ g \circ f_R \xrightarrow{\alpha} h_R \circ i \circ f \circ f_R \rightarrow h_R \circ i
\]
\begin{Definition}
A square as in \eqref{bcsquarebefore} with 2-morphism $\alpha$ is said to satisfy the right \emph{Beck-Chevalley condition} if $\alpha_R$ is invertible.
\end{Definition}
Similarly, if the horizontals $g,i$ both have left adjoints, we can define the left Beck-Chevalley condition via the left mate square
\[
\tik
A\arrow[]{d}{f} & B\arrow[dashed,red,thick]{l}[above]{g_L} \arrow[]{d}{h}  \\ 
C  & D\arrow[dashed,red,thick]{l}[below]{i_L} \arrow[red,shorten >=0.4cm,shorten <=0.4cm,Rightarrow]{ul}[above,sloped]{\alpha_L}
\tak
\]
\begin{Remark}
Note that a square satisfies the right BC condition iff it satisfies the left BC condition, when both are defined, hence we can omit the words \emph{left} or \emph{right}.
\end{Remark}

To get relations between mates of squares we need to look at cubes.

\begin{Lemma}
\label{lem:cubemate}
Consider a commutative cube (see \autoref{app:commcube} for details)
\begin{align*}
\stik{0.7}{
{} \& {} \& {}\\
{} \ar{ur}{\scalebox{2}{$z$}} \ar{rr}{\scalebox{2}{$x$}} \ar{dd}{\scalebox{2}{$y$}} \& {} \& {}\\
{} \& {} \& {} \\
{} \& {} \& {}
}
&
{}
&
\stik{0.7}{
{} \& {} \ar{rr}[name=topback,below]{} \ar{dd}[name=backleft,sloped,xshift=-1.5pc]{} \& {} \& {} \ar{dd}\\
{} \ar[crossing over]{rr}[name=topfront,above]{}\ar{dd}[name=frontleft]{} \ar{ur}[name=topleft,below]{} \& {} \& {} \ar{dd}[name=frontright,sloped,xshift=1pc]{} \ar{ur}[name=topright,below]{} \& {}\\
{} \& {} \ar{rr} \& {} \& {}\\
{} \ar{rr}[name=bottomfront,below]{} \ar{ur}[name=bottomleft,sloped,yshift=-0.2pc]{} \& {} \& {} \ar{ur}
\arrow[Rightarrow,to path={(topright) to[bend left] (topback)}]{}{}
\arrow[Rightarrow,to path={(frontright) to[bend right] (bottomfront)}]{}{}
\arrow[Rightarrow,crossing over,to path={(frontright) to[bend right] (topright)}]{}{}
\arrow[Rightarrow,to path={(bottomfront) to[bend right] (bottomleft)}]{}{}
\arrow[Rightarrow,to path={(bottomleft) to[bend left] (backleft)}]{}{}
\arrow[Rightarrow,to path={(topback) to[bend left] (backleft)}]{}{}
\latearrow{/tikz/commutative diagrams/crossing over}{2-3}{4-3}{}
\latearrow{/tikz/commutative diagrams/crossing over}{2-1}{2-3}{}
\latearrow{/tikz/commutative diagrams/crossing over}{2-3}{1-4}{}
}
\end{align*}
and suppose that all arrows in the $x$ (resp. $z$) direction have left (resp. right) adjoints, with given unit/counit. Then the left (right) mate of the cube, i.e. the cube obtained from taking the left (right) mates of all faces involving direction $x$ ($z$) arrows, commutes. Explicitly, they are the following cubes
\begin{align*}
\stik{0.7}{
{} \& {} \& {} \& {} \& {}\\
{} \& {} \& {} \ar{ur}{\scalebox{2}{$z$}} \ar[dashed,red,thick]{ll}[above]{\scalebox{2}{$x_L$}} \ar{dd}{\scalebox{2}{$y$}} \& {} \& {}\\
{} \& {} \& {} \& {} \& {} \\
{} \& {} \& {} \& {} \& {}
}
&
{}
&
\stik{0.8}{
{} \& {} \ar[leftarrow,dashed,red,thick]{rr}[name=topback,below]{} \ar{dd}[name=backleft,sloped,xshift=-1.5pc]{} \& {} \& {} \ar{dd}[name=backright,sloped,left]{}\\
{} \ar[leftarrow,dashed,red,thick,crossing over]{rr}[name=topfront,above]{}\ar{dd}[name=frontleft]{} \ar{ur}[name=topleft,below,sloped,xshift=0.5pc]{} \& {} \& {} \ar{dd}[name=frontright,sloped,xshift=1pc]{} \ar{ur}[name=topright,below]{} \& {}\\
{} \& {} \ar[leftarrow,dashed,red,thick]{rr}[name=bottomback,above]{} \& {} \& {}\\
{} \ar[leftarrow,dashed,red,thick]{rr}[name=bottomfront,above]{} \ar{ur}[name=bottomleft,sloped,yshift=-0.2pc]{} \& {} \& {} \ar{ur}[name=bottomright,sloped,above]{}
\arrow[Rightarrow,red,to path={(bottomright) to[bend right] (bottomfront)}]{}{}
\arrow[Rightarrow,red,crossing over,to path={(bottomfront) to[bend right] (frontleft)}]{}{}
\arrow[Rightarrow,to path={(frontleft) to[bend right] (topleft)}]{}{}
\arrow[Rightarrow,crossing over,to path={(bottomright) to[bend left] (backright)}]{}{}
\arrow[Rightarrow,red,to path={(backright) to[bend left] (topback)}]{}{}
\arrow[Rightarrow,red,crossing over,to path={(topback) to[bend left] (topleft)}]{}{}
\latearrow{/tikz/commutative diagrams/crossing over}{2-3}{4-3}{}
\latearrow{/tikz/commutative diagrams/leftarrow,dashed,red,thick,/tikz/commutative diagrams/crossing over}{2-1}{2-3}{}
\latearrow{/tikz/commutative diagrams/crossing over}{2-3}{1-4}{}
} \\
\stik{0.7}{
{} \& {} \& {} \& {} \& {}\\
{} \& {} \& {} \ar[dashed,thick,blue]{dl}[above,xshift=-0.5pc]{\scalebox{2}{$z_R$}} \ar{rr}[above]{\scalebox{2}{$x$}} \ar{dd}{\scalebox{2}{$y$}} \& {} \& {}\\
{} \& {} \& {} \& {} \& {} \\
{} \& {} \& {} \& {} \& {}
}
&
{}
&
\stik{0.8}{
{} \& {} \ar{rr}[name=topback,below]{} \ar{dd}[name=backleft,sloped,xshift=-1.5pc]{} \& {} \& {} \ar{dd}[name=backright,sloped,left,xshift=0.5pc]{}\\
{} \ar[crossing over]{rr}[name=topfront,below,xshift=1pc]{} \ar{dd}[name=frontleft,sloped,xshift=-1pc]{} \ar[leftarrow,dashed,blue,thick]{ur}[name=topleft,above,sloped,xshift=0.5pc]{} \& {} \& {} \ar{dd}[name=frontright,sloped,xshift=1pc]{} \ar[leftarrow,dashed,blue,thick]{ur}[name=topright,above]{} \& {}\\
{} \& {} \ar{rr}[name=bottomback,above,xshift=-1pc]{} \& {} \& {}\\
{} \ar{rr}[name=bottomfront,above]{} \ar[leftarrow,dashed,blue,thick]{ur}[name=bottomleft,sloped,right]{} \& {} \& {} \ar[leftarrow,dashed,blue,thick]{ur}[name=bottomright,sloped,below]{}
\arrow[Rightarrow,to path={(backright) to[bend right] (bottomback)}]{}{}
\arrow[Rightarrow,blue,to path={(frontleft) to[bend left] (bottomleft)}]{}{}
\arrow[Rightarrow,blue,to path={(bottomleft) to[bend right] (bottomback)}]{}{}
\arrow[Rightarrow,blue,to path={(topfront) to[bend left] (topright)}]{}{}
\arrow[Rightarrow,blue,to path={(topright) to[bend right] (backright)}]{}{}
\arrow[Rightarrow,crossing over,to path={(topfront) to[bend left] (frontleft)}]{}{}
\latearrow{/tikz/commutative diagrams/crossing over}{2-3}{4-3}{}
\latearrow{/tikz/commutative diagrams/crossing over}{2-1}{2-3}{}
\latearrow{/tikz/commutative diagrams/leftarrow,dashed,blue,thick,/tikz/commutative diagrams/crossing over}{2-3}{1-4}{}
\latearrow{/tikz/commutative diagrams/leftarrow,dashed,blue,thick}{4-3}{3-4}{}
}
\end{align*}
Using the description from Appendix $\ref{app:commcube}$ the first cube corresponds to the ordering of coordinates $y<z<x$ and the second to the ordering $z<x<y$.
\end{Lemma}
\begin{proof}
In a 2-category this is a direct computation, using the 4-interchange law, and the fact that the original cube commutes. 
\end{proof}

\section{Adjunction of inverse and direct image for sheaves on finite sets}
\label{app:pullpushadjsets}
Let $\varphi:S\rightarrow T$ be a map of sets, and let $\varphi^*,\varphi_*$ be the functors of inverse and direct image between the categories of sheaves. Let $V\in\Sh(S),W\in\Sh(T),A\subset S,B\subset T$. Note that for a sheaf on a finite set we have \[
V(A)=\prod_{a\in A}V_a
\]
so we have the following formulas:
\begin{gather}
\varphi^*W(A)=\prod_{a\in A}W_{\varphi(a)}\\
\varphi_*V(B)=V(\varphi^{-1}(B))
\end{gather}
and so
\begin{gather}
\varphi^*\varphi_*V(A)=\prod_{a\in A}V(\varphi^{-1}(\varphi(a)))\\
\varphi_*\varphi^*W(B)=\prod_{a,\varphi(a)\in B}W_{\varphi(a)}
\end{gather}
The unit and counit of the adjunction $\varphi^*\dashv\varphi_*$ are given by maps
\begin{gather}
\epsilon_R: \varphi^*\varphi_*V(A)=\prod_{a\in A}V(\varphi^{-1}(\varphi(a))) \rightarrow \prod_{a\in A}V_a=V(A)\\
\eta_R: W(B)=\prod_{b\in B}W_b\rightarrow \prod_{a,\varphi(a)\in B}W_{\varphi(a)}=\varphi_*\varphi^*W(B)
\end{gather}
where $\epsilon_R$ is given by restrictions and $\eta_R$ by the diagonal maps.

There is also an adjunction $\varphi_*\dashv\varphi^*$ given by maps
\begin{gather}
\eta_L: \varphi^*\varphi_*V(A)=\prod_{a\in A}V(\varphi^{-1}(\varphi(a))) \leftarrow \prod_{a\in A}V_a=V(A)\\
\epsilon_L: W(B)=\prod_{b\in B}W_b\leftarrow \prod_{a,\varphi(a)\in B}W_{\varphi(a)}=\varphi_*\varphi^*W(B)
\end{gather}
where $\eta_L$ is given by extension by 0, and $\epsilon_L$ is given by the sum maps.

%%%%%%%%%%%%%%%%%%%%%%%%%%%%%%%%%%%%%%%%%%%%%%%%%%%%%%%%%
%%%%%%%%%%%%%%%%%%%%%%%%%%%%%%%%%%%%%%%%%%%%%%%%%%%%%%%%%

\section{Limits}
\label{app:PBcont}

\subsection{Weak adjoints}
\begin{Definition}[see \cite{Gray2adj}]
Let $F:\CCC\rightarrow\DDD$, $G:\DDD\rightarrow\CCC$ be functors of bi-categories, then we say that $G$ is \emph{weak right adjoint} to $G$ if there is a natural functor
\[
\Hom(FC,D)\leftarrow\Hom(C,GD)
\]
which admits a right adjoint.
\end{Definition}

We will mostly be interested in the case where $\DDD$ is trivial, where this amounts to saying that we have some chosen object $G(\point)$, and for any $C$ the map $\Hom(C,G(\point))\rightarrow \point$ has a right adjoint, which is the same as saying that $\Hom(C,G(\point))$ has a final object. 
\subsection{Conical limits}
Let $K$ be a small 1-category and $\CCC$ a 1-category.

Let $F:K\rightarrow \CCC$ be a functor. The limit of $F$ can be thought of as follows (cf. \cite{grandisparedouble}):

Denote also by $F$ the functor $\point\rightarrow\CCC^K$ which sends $\point$ to $F$, and by $diag$ the diagonal embedding $\CCC\rightarrow\CCC^K$. Then we may form the comma category
\[
\stik{1}{
(diag\downarrow F) \ar{d} \ar{r}[above]{p} \& \CCC   \ar{d}{diag}\\
\point \ar{r}{F} \&  \CCC^K
}
\]
Note that a final object $L$ in $(diag\downarrow F)$ is exactly a limit of $F$ together with all the relevant morphisms to the diagram. If we want just the object, then it is given by $p(L)$. So the condition of having a limit is the same as the requirement that $(diag\downarrow F)$ has a final object, which is the same as requiring that the map  $(diag\downarrow F)\rightarrow \point$ has a right adjoint.

\subsection{Weak limits and \comma squares}
\label{app:WeightedLimits}
In the above, we only dealt with conical limits, i.e. we used the map $\CCC\xrightarrow{diag}\CCC^K$ which comes from the map $K\rightarrow\point$.

However, we can replace it by any map $K\xrightarrow{W} L$, and form the square
\[
\stik{1}{
(W^*\downarrow F) \ar{d} \ar{r}[above]{p} \& \CCC   \ar{d}{W^*}\\
\point \ar{r}{F} \&  \CCC^K
}
\]
We now say that $F$ admits a $W$-limit if the map $(W\downarrow F)\rightarrow \point$ admits a weak right adjoint (this is closely related to the notion of \emph{weighted} limit appearing in the literature).

\begin{Example}[\comma Squares]
Let $K\rightarrow L$ be the map 
\[
\stik{1}{
{} \&  \bullet\ar{d} \\
 \bullet\ar{r} \& \bullet
}
\xhookrightarrow{W}
\stik{1}{
 \bullet \ar{r} \ar{d} \&  \bullet\ar{d} \ar[Rightarrow,shorten <=0.7em,shorten >=0.7em]{dl}\\
 \bullet\ar{r} \& \bullet
}
\]
and let $\CCC$ be a bicategory. 

A map $K\xrightarrow{F}\CCC$ is a "bottom right corner", and we call a $W$-limit of $F$ an \comma square with this bottom right corner (if $\CCC$ is a 1-category this conicides with the usual notion of Cartesian square).
\end{Example}

Let us analyze this in more detail:

Let $F=\stik{1}{
{} \&  A\ar{d}{f} \\
B\ar{r}{g} \& C
}$ be a bottom right corner in $\CCC$, and consider the square:
\[
\stik{1}{
(W^*\downarrow F) \ar{d} \ar{r}[above]{p} \& \CCC^\square  \ar{d}{W^*}\\
\point \ar{r}{F} \&  \CCC^\lrcorner
}
\]

Objects of $(W^*\downarrow F)$ are pairs $(S\in \CCC^\square,\alpha:W^*S\rightarrow F)$. So they can be thought of as diagrams:
\[
\stik{0.7}{
{} \& Z \ar{rr}[name=topback,below]{} \ar{dd}[name=backleft,sloped,xshift=-1.5pc]{} \& {} \& W \ar{dd}\\
X \ar[crossing over]{rr}[name=topfront,above]{} \ar{ur}[name=topleft,below]{} \& {} \& Y \ar{dd}[name=frontright,sloped,xshift=1pc]{} \ar{ur}[name=topright,below]{} \& {}\\
{} \& B \ar{rr} \& {} \& C\\
 \& {} \& A \ar{ur}
\arrow[Rightarrow,to path={(topright) to[bend left] (topback)}]{}{}
\arrow[Rightarrow,crossing over,to path={(frontright) to[bend right] (topright)}]{}{}
\arrow[Rightarrow,to path={(topback) to[bend left] (backleft)}]{}{}
\latearrow{/tikz/commutative diagrams/crossing over}{2-3}{4-3}{}
\latearrow{/tikz/commutative diagrams/crossing over}{2-1}{2-3}{}
\latearrow{/tikz/commutative diagrams/crossing over}{2-3}{1-4}{}
}
\]
A morphism in  $(W^*\downarrow F)$ is then a commutative diagram
\[
\stik{0.7}{
{} \& Z' \ar{rr} \ar{dd} \& {} \& W' \ar{dd}\\
X' \ar[crossing over]{rr} \ar{dd} \ar{ur} \& {} \& Y' \ar{dd} \ar{ur} \& {}\\
{} \& Z \ar{rr}[name=topback,below]{} \ar{dd}[name=backleft,sloped,xshift=-1.5pc]{} \& {} \& W \ar{dd}\\
X \ar[crossing over]{rr}[name=topfront,above]{} \ar{ur}[name=topleft,below]{} \& {} \& Y \ar{dd}[name=frontright,sloped,xshift=1pc]{} \ar{ur}[name=topright,below]{} \& {}\\
{} \& B \ar{rr} \& {} \& C\\
 \& {} \& A \ar{ur}
}
\]
together with a map
\[
\stik{0.7}{
{} \& Z' \ar{rr} \ar{dd} \& {} \& W' \ar{dd}\\
 \& {} \& Y' \ar{dd} \ar{ur} \& {}\\
{} \& Z \ar{rr}[name=topback,below]{} \ar{dd}[name=backleft,sloped,xshift=-1.5pc]{} \& {} \& W \ar{dd}\\
 \& {} \& Y \ar{dd}[name=frontright,sloped,xshift=1pc]{} \ar{ur}[name=topright,below]{} \& {}\\
{} \& B \ar{rr} \& {} \& C\\
 \& {} \& A \ar{ur}
} \rightarrow \stik{1}{
{} \& Z' \ar{rr}[name=topback,below]{} \ar{dd}[name=backleft,sloped,xshift=-1.5pc]{} \& {} \& W' \ar{dd}\\
 \& {} \& Y' \ar{dd}[name=frontright,sloped,xshift=1pc]{} \ar{ur}[name=topright,below]{} \& {}\\
{} \& B \ar{rr} \& {} \& C\\
 \& {} \& A \ar{ur}
}
\]
